# Supplementary material for: Tropical $\psi$ classes
Source: arXiv:2009.00586 source file (2020-09-02)
Supplement: Supplementary file 1 [file appendix.tex]

\appendix
\addtocontents{toc}{\protect\setcounter{tocdepth}{1}}

https://www.overleaf.com/project/5c4a08e0f786bc0dbd391a04
\section{Project outline}

\rcolor{After discussing with Andreas last week, I want to try and slightly adapt the scope of this project. My initial understanding was that we would not mess at all with tropical intersection theory, and just take a stack theoretic perspective to be able to use it off the shelf. The major obstacle here is that it seems extremely artificial to select a class of families of tropical curves that are well behaved without essentially asking such families to come from geometry (stable maps or admissible covers). Andreas convinced me that we should instead think of tropical $\psi$ as being a Chern class evaluated on a stack, i.e. something that can be evaluated on relatively arbitrary tropical families. Then the correspondence theorem happens when we evaluate them on families coming from geometry. Here is my list of what material should be developed.}

\begin{description}
\item[intersection theory] this is the foundational part that Andreas is developing. If I understand correctly, we are not reinventing tropical intersection theory, but reformulating it in a way that is better tuned to our purposes (i.e. to be applied to families of curves). Abstract tropical varieties are endowed with sheaves of affine linear functions, and differential forms. Morphisms of tropical objects should preserve this structure.
Then one should be able to define cycles, pull-backs and push-forwards, and first chern classes of line bundles. It is not completely clear to me, and it should probably be the focus of the next discussion with Andreas, how much of this is already in some form in place.  
\item[families of curves] one wants to define a notion of good family of tropical curves: a piecewise linear function among tropical spaces, where the fibers are tropical curves and there is a natural short exact sequence induced on the sheaves of differential forms, saying the differential forms on the total space of the family should be an extension of forms on the base and forms on the fiber. With this definition of family of tropical curves, there will be many families which are tropical, but not the tropicalization of classical families. We want to think of this as a feature and not a bug.
\item[smooth vs. non-smooth families] right now Andreas is making definitions where all weights of top dimensional cells in both the base and the fiber curves are equal to one. I feel we might need to enlarge this to contain a set-up for higher weights, for the simple reason that most of the families offered to us by geometry are such, as Hannah and I realized in Tubingen. I am not sure whether such a generalization is only technical, or  if it has conceptual obstructions. This should be anothe discussion.
\item[$\psi$ class] the $\psi$ class can be defined as the negative self intersection of a section for a family of tropical curves. If we have a good theory of line bundles and their chern classes, we may want to define the cotangent line bundle for a family of curves, using our sheaves of differential forms to give transition functions. In this context, $\psi$ on $M_{1.1}^{trop}$ is not in any natural way $1/24$[pt.], but rather a way to assign a number to any one dimensional good family of tropical curves.
\item[formal properties of $\psi$ classes] We would still want to show the formal pull back and pushforward relations of $\psi$ classes. Andreas gave a sketch of an argument in Oberwolfach for the pull-back relation. What seems to drive everything is that the tautological relations should be able to be checked locally.
\item[geometric correspondence] Note that up to here, there is no real need to restrict to genus $1$. We are so far describing a pretty general theory. But of course I think we need to give some applications for this theory. If the above parts all work out, I feel the geometric applications that would be whithin reach are:
\begin{itemize}
    \item genus $1$ well-spaced stable maps to a surface. (Linear pencils on smooth surfaces is the case we essentially checked in Tubingen. For more interesting cycles we need to have in place the theory of spaces with weights on cells).
    \item Admissible covers spaces. Here I think we could even go beyond genus $1$ and we should essentially find a very similar theory to Zhi (Mark Gross's student).
\end{itemize}

\end{description}

\renzo{I am going to take the approach of writing in blue anything which is in preliminary stage, where I want to put down some idea but will probably want to reformulate and polish it before it is sharable outside our group.}

\rcolor{A theory of tropical $\psi$ classes exists in genus zero (cite Allermann-Markwig, Rau, Katz). 
It is simultaneously a purely combinatorial theory, and a mirror of the classical theory via the "operational"/toric intersection theory point of view. By this I mean
\begin{equation}
    \prod(\psi_i^{trop})^{k_i} = \sum \left(\prod \psi_i^{k_i}\cdot \Delta_\tau \right) \tau,
\end{equation}
where $\tau$ ranges among all cones of $M_{0,n}^{trop}$.

What makes everything tick in genus $0$ is that $M_{0,n}^{trop}$ is naturally embedded in $\R^N$ as a balanced fan, and one can use tools of toric/tropical intersection theory (mention Fulton-Sturmfels, Katz, ...?).
For higher genus, such an embedding is not possible. At a very basic level, $\Mt{1,1}$ consists of a single ray, which as such may not possibly become a balanced fan. \footnote{See  \ref{p24}.}

\noindent{\textsc{Step 1: defining the theory:}}

The idea would be to exploit the fact that moduli space of tropical curves have been given a stack structure in (cite CCUW)that makes them into fine moduli spaces. We therefore want to use the philosophy that any geometric concept on a stack may be defined by looking at all of its pullbacks from representable maps from schemes to the stack. 

In our specific case, we are concerned with maps:
$$
f:C \to \mt{1,n},
$$
where $C$ belongs to a class $\calC$ of well behaved tropical objects, and $f$ should be representable in the sense that the family $X_f$ should also belong to the class $\calC$.
\vspace{0.2cm}

Ideally we would like to give a fairly slick and general definition of $\calC$ along the lines of: { \it $C\in \calC$ is a {\bf balanced} (or locally balanced?) (extended?, generalized?) cone complex}. We also may want to describe the notion of local-balancing in terms of a sheaf of groups whose sections  we interpret as the restriction of linear functions from an ambient space to the cone complex. 
\vspace{0.2cm}

But as a {\bf minimal requirement} we would like to make sure that our definitions include {\bf realizable} families of tropical stable maps to toric targets, where the base of the family may need to be given a balanced structure as additional information. {\it The idea here is the following. Allow me the abuse of language to call "horizontal" any direction that has to do with the base of the family, and "vertical" what relates to fiber. Horizontal balancing may need to be provided, but the vertical balancing should then be induced by the vector space structure of the target space $\R^n$.}

We also want the following forgetful morphisms to be representable:
$$
\mt{1,n}(\R^N, \Delta)\to \mt{1, n+|\Delta|}
$$
and
$$
\mt{1,n+1}\to \mt{1, n}.
$$

Then tropical $\psi$ classes may be defined as follows:
for any diagram where $f$ is a "good" map,
$$
\xymatrix{
\Gamma \ar[d]^\pi & \\
C \ar[r]^{f} \ar@/^1pc/[u]^s & \mt{1,n}
}
$$
 define 
\begin{equation} \label{defpsi}
f^\ast\psi:= -\pi_\star (Im(s)^2).    
\end{equation}

This prescription should define $\psi$ on the stack! Further it should be sufficient to describe $f^\ast \psi$:
\begin{itemize}
    \item for one good atlas (i.e. $f$ surjective), OR
    \item for enough curves mapping into the stack,
\end{itemize}
to completely determine $\psi$.

\vspace{0.2cm}
{\it
\noindent{\bf Observations to ourselves:}
\begin{itemize}
    \item To show the compatibility among various test family it should be feasible to show that the category $\calC$ we defined admits fiber products.
    \item The families to $\mt{1,1}$ that we have been studying give an atlas for $\mt{1,1}$ are certainly surjective. Are the fiber product with forgetful morphisms $\mt{1,n+1}\to \mt{1, n}$ also surjective? (I want to say so). Are they realizable? (I also want to say so: the question now boils down to whether attaching a contracting tree to a realizable genus $1$ tropical curve messes with realizability - again the gut feeling is that it shouldn't but this needs to be carefully checked).
\end{itemize}}

Once we have defined tropical $psi$ classes this way, similarly we could define intersection cycles by:
$$
f^\star \psi^I: = (f^\star \psi)^I
$$
(the RHS of this equation lives on $C$ where we know how to do intersection theory).

At this point we will have defined a tropical theory of  $\psi$ classes and their intersections (which by the way is quite possibly a viable definition for genus higher than $1$.) 
All of this should be fleshed out and detailed in Section \ref{brm}

\noindent{\textsc{Step 2: computing the theory:}}

In order to compute the theory, the hope is to have a two step approach: first we compute the degree of the class $\psi_1$ on $\mt{1,1}$ to be $\frac{1}{24}[v]$ {\it (there is an interesting question here whether the vertex of $\mt{1,1}$ should carry a $B\mu_2$ structure like the generic point on the ray or not. However this seems  something that we can save for later).}

We choose as an atlas for $\mt{1,1}$ a one-dimensional family of realizable tropical stable maps of degree three to the tropical projective plane, passing through $8$ fixed general points:
\begin{equation}
   [\gamma_f] =  \prod_{i=1}^8 ev_i^\ast (P_i)_{|[\calR\mt{1, 8}(\TT\PP^2, 3)]}\in A^1(\mt{1, 8}(\TT\PP^2, 3)) .
\end{equation}
(here we are denoting by $\calR\mt{1, 8}(\TT\PP^2, 3)]$ the representable locus in the moduli space of tropical stable maps, which is thought somehow like a virtual class). 

The above cycle arises from a map 
\begin{equation}
    f: T \to \mt{1,1},
\end{equation}
where $T$ is a trivalent tree endowed {\it by us and by declaration, I suppose} with the standard balanced local structure.
In Section \ref{tf} we study in detail the map $f$ arising when we choose the points $P_i$ to be in horizontally stretched position, compute the degree of the map to be $12$
and the self intersection of a section to be $-1$, thus recovering via a purely tropical intersection theoretic computation the degree of $\psi_1$ to be $1/24$ (It is $1/12$ the class of a point on the ray of $mt{1,1}$, which carries a $B\mu_2$ structure.)

We of course want to test this computation for consistency, and we do so by observing that the computation is unchanged with respect to the following choices:
\begin{itemize}
    \item Any of the $8$ sections available as fixed points in the family.
    \item We also analyze a different one dimensional family of maps (where the way to get a $12$ is $3+1+\ldots +1$.
    \item Q: What about tropical sections arising from the boundary contacts? Are they essentially different creatures because they are attached to points with nontrivial log structure, or can we frame them into a similar story?
\end{itemize}
{\it Of course all of these consistency checks are crucially important in terms of leading us to a general proof of independence of choices, but once we have that and feel solid about it, this can all be just omitted or mentioned in passing.}

To compute the theory for more points and in higher codimension, we of course do not want to rely on explicit computations, but rather on the development of tatutological relations. In fact it would suffice to establish the tropical version of:
\begin{description}
\item[pull-back] the pull-back relation
$$
\psi_i = \pi_{n+1}^\ast(\psi_i) + S_i,
$$
where $S_i$ is a suitable version of a cycle arising from the $i$-th section. See \ref{} for more discussion.
\item[string]
$$
 \pi_{n+1, \ast} \prod_{i=1}^n \psi_i^{k_i} = \sum_{j=1}^n \psi_j^{k_j-1}\prod_{i\not=j} \psi_i^{k_i}.
$$
\item[dilaton]
$$
 \pi_{n+1, \ast}\left(\psi_{n+1}\prod_{i=1}^n \psi_i^{k_i}\right) =n\prod_{i=1}^n \psi_i^{k_i}.
$$
\end{description}
The resulting theory should be an operational theory which is very similar to the genus zero theory. The operational class $\psi_i$
should be expressed as a tropical cycle as the sum of all cones where the $i$-th points lies on a four-valent, genus zero vertex.

In a sense, this is the theory that we would want to begin with, but the main contribution of this work is to make such a theory arise from tropical intersection theoretic considerations, as opposed to just being a definition.

\noindent{\bf Question/Remark:} Is this result a manifestation of the fact that the tautological ring in genus one is completely supported on the boundary? 

\noindent{\bf Observation:} the real technical obstruction to going besides genus $1$ is the lack of understanding of the realizability condition in higher genus. We do not have an analogue of well-spacedness, and therefore can't impose a tropical condition that makes the families of tropical curves equidimensional and balanceable.
}
\section{Balancing and  Representable Morphisms}\label{brm}

What this definitions are meant to model are just the notion of local balancing. The goal is to express the fact that a tropical object admits a local embedding into a vector space without mentioning those words.

\begin{definition}
An {\bf abstract, locally balanced, tropical curve} is a tropical curve $\Gamma$ together with a sheaf $\calO_\Gamma$ of finitely generated abelian groups, satisfying the following axioms:
\begin{enumerate}
    \item the stalk at a vertex $v$ is a subgroup $\calO_{\Gamma,v} \hookrightarrow \ZZ^{val(v)} = \oplus_{e\to v} \ZZ \cdot e$;
    \item for any non-empty open set $U$ which is completely contained in an edge $e$ we have $\calO_{\Gamma}(U)\hookrightarrow \ZZ = \Z\cdot e$. We denote by $\calO_{\Gamma,e}$ the stalk at any point in the interior of an edge $e$.
    \item There exists a map $w: E(\Gamma)\to \N$, such that, for every $e\to v$ the maps $\varphi_{e,v}:\calO_{\Gamma,v}\to \calO_{\Gamma,e}$ are given by composition of the inclusion from $(1)$ and the scaling of a linear  projection by $w(e)$ as in the diagram:
   \begin{equation}
      \xymatrix{
    \calO_{\Gamma,v} \ar@{^{(}->}[r] \ar[d]_{\varphi_{e,v}} &\bigoplus_{\tilde{e}\to v} \ZZ \cdot \tilde{e} \ar[d]^{w(e)\pi_e}\\
      \calO_{\Gamma,e} \ar@{^{(}->}[r]&\ZZ 
     }  
   \end{equation}
   \item For every vertex $v$, we have
   \begin{equation}
       \sum_{e\to v} \varphi_{e,v} = 0.
   \end{equation}
\end{enumerate}

$\calO_\Gamma$ is called the sheaf of linear functions of $\Gamma$. The curve $\Gamma$ is called {\bf smooth} if $Im(w) = \{1\}$.  
\end{definition}
\renzo{I don't like this very much, the weight stuff should actually be recoverable directly from the embedding of the functions into the free abelian groups}
Second try:

\begin{definition}
An {\bf abstract, locally balanced, tropical curve} is a tropical curve $\Gamma$ together with a sheaf $\bals_\Gamma$ of finitely generated abelian groups, satisfying the following axioms:
\begin{enumerate}
    \item the stalk at a vertex $v$ is a subgroup $\bals_{\Gamma,v} \hookrightarrow \ZZ^{val(v)} = \oplus_{e\to v} \ZZ \cdot e$;
    \item for any non-empty open set $U$ which is completely contained in an edge $e$ we have $\bals_{\Gamma}(U)\hookrightarrow \ZZ = \Z\cdot e$. We denote by $\bals_{\Gamma,e}$ the stalk at any point in the interior of an edge $e$.
    \item  for every $e\to v$ the maps $\varphi_{e,v}:\bals_{\Gamma,v}\to \bals_{\Gamma,e}$ are given by  the linear  projection on $\ZZ\cdot e$ as in the diagram:
   \begin{equation}
      \xymatrix{
    \bals_{\Gamma,v} \ar@{^{(}->}[r] \ar[d]_{\varphi_{e,v}} &\bigoplus_{\tilde{e}\to v} \ZZ \cdot \tilde{e} \ar[d]^{\pi_e}\\
      \bals_{\Gamma,e} \ar@{^{(}->}[r]&\ZZ 
     }  
   \end{equation}

   \item For every vertex $v$, we have
   \begin{equation}
       \sum_{e\to v} \varphi_{e,v} = 0.
   \end{equation}
\end{enumerate}

$\bals_\Gamma$ is called the {\bf local balancing sheaf} of $\Gamma$. The curve $\Gamma$ is called {\bf smooth} if all maps $\varphi_{e,v}$ are onto.  
\end{definition}

\renzo{I think this definition now mimicks the traditional  local balancing. I am a little hesitant in calling it cotangent sheaf because this is not an intrinsic sheaf attached to a tropical curve. The same tropical curve could be embedded in different vector spaces yielding non-isomorphic balancing sheaves. However we can rename it in a way which is more consistent with the literature.}

\section{Balancing rebooted}
\renzo{
I want to define a notion of local balancing of a rational polyhedral complex $\Gamma$ in terms of a sheaf on $\Gamma$, but in terms of a topology which reflects the topology of the dual (classical) algebraic objects.
}

\begin{definition}
Let $\Gamma$ be a locally finite RPC. We define a subcomplex $U$ of $\Gamma$ to be an open set if whenever a polyhedron $\sigma$ is inside $U$, then all of its faces are also in $U$.
The collection of all such open sets defines a topology on $\Gamma$,\rcolor{which probably is well known and has a name in some circles.}
\end{definition}

\renzo{Informally, open sets are closed subcomplexes in the Euclidean topology. So individual vertices are open sets, edges together with their endpoints, etc... }

\begin{definition}
A sheaf $\calB$ on $\Gamma$ is a {\bf local balancing sheaf} if:
\begin{enumerate}
    \item For every closed polyhedron $\sigma$
    $$
    \calB(\sigma)\subseteq H \subset \bZ^{\star(\sigma)},
    $$
    where $H = \{\sum x_i = 0\}$ denotes the hyperplane of points whose coordinates add to $0$.
    \item If $\tau$ is a face of $\sigma$,
    $$
    \calB(\sigma) \to W \subseteq \calB(\tau)
    $$
    is an inclusion, and it factors through the subspace
    $W\subset \bZ^{\star(\tau) }$ spanned by the cones in $\star(\tau)$ which do not belong to $\sigma$.
\end{enumerate}
\end{definition}
\renzo{ Some observations:
\begin{itemize}
    \item In (2), $\tau$ needs not be a codimension one face of $\sigma$. If $\tau$ is codimension one then $\sigma$ is the unique cone in $\star(\tau)$ contained in $\sigma$, hence we are setting exactly one coordinate equal to zero. 
    \item This data should be equivalent to the existence of local balanced embeddings in a vector space around any polyhedron $\sigma$, or, if you want, the existence of a global balanced embedding of the universal cover of $\Gamma$ in a (possibly infinite dimensional) vector space. \item I am being a little sloppy with lattice vs. vector space language. Some statements need to be about lattices (e.g we need to be the functions to be integral), but some statements are more natural in terms of vector spaces (e.g. defining $W$).
    \item If $\Gamma$ is (locally around $\sigma$) embedded in a vector space $V$, and $\tau$ is a face of $\sigma$, then we have the following inclusions:
    $$
    \langle \tau \rangle_{\RR} \subseteq   \langle \sigma \rangle_{\RR} \subseteq   \langle \star(\sigma) \rangle_{\RR} \subseteq   \langle \star(\tau) \rangle_{\RR} \subseteq V.
    $$
    
\end{itemize}
}

\section{Test Families for $\psi_1$ on $M_{1,1}^{trop}$}\label{tf}

\subsection{$12=4+1+\ldots+1$}
Fix $8$ points in horizontally stretched position. We study the map $$f:T\to \mt{1,1}$$ for the one-dimensional family $T$ of cubics passing through the $8$ points.

We first consider the fiber of $f$ for a point in $\mt{1,1}$ which corresponds to a curve with a very large $j$-invariant.
By \rcolor{cite} Kerber-Markwig, any curve in the fiber has a contracted edge, and can be interpreted as a \rcolor{singular/nodal} rational curve if we remove the contracted edge.
We thus have to consider the 12 rational cubics passing through the 8 points, and understand how they arise as elliptic cubics with a large $j$-invariant.

$8$ of those curves are of multiplicity $1$. They each have a crossing, i.e.\ a parallelogram in the dual subdivision. It is this crossing where we can hide a contracted bounded edge.

We can compute the degree of the map $ev\times j$ for this curve, and it is one.

There is one more rational cubic, of multiplicity $4$, which contains a bounded edge with weight $2$. Following our discussions with Dhruv, we can add a contracted edge as a loop in the middle of the weight $2$ edge to be realizable. The $ev\times j$-multiplicity is then $8$, and we believe that the contracted loop produces an automorphism factor of $\frac{1}{2}$, so that we obtain $4$ in total.

Now we study the fiber of $f$ for a point in $\mt{1,1}$ with a very small $j$-invariant. Now the curves are degenerations of the $12$ rational curves, where we introduce a small cycle. For any of the multiplicity-$1$-curves with the crossing, it is not possible to introduce a small cycle.
For the multiplicity-$4$-curve with the weight $2$ edge, we can again have a tiny loop in the middle of the edge, or a tiny flat cycle in the middle of the edge. We already computed the $ev\times j$-multiplicity of the first times the automorphism factor to be $4$. For the second, we compute the $ev\times j$-multiplicity to be $16$. Again, we believe that there is an automorphism factor of $\frac{1}{2}$ in charge of exchanging the two indistinguishable edges forming the flat cycle.

As we shrink the $j$-invariant to $0$, the two curves become equal.

To sum up, the map has a single preimage over the vertex of $\mt{1,1}$, which splits into two edges of multiplicity $4$ and $8$, respectively. The multiplicity $4$-edge is an end. The multiplicity-$8$-edge splits further and eventually ends up being $8$ multiplicity-$1$-ends over points with a very large $j$-invariant.

\subsection{$12=3+1+\ldots+1$}
We pick another point configuration \rcolor{reference}, such that the $12$ rational curves through them consist of one curve of multiplicity $3$ (containing an area-$3$-triangle in its dual subdivision, with vertices $(0,0)$, $(1,2)$, $(2,1)$ and interior point $(1,1)$) and $9$ curves of multiplicity $1$, which as before each have a crossing of edges dual to a parallelogram. 

The fiber over a point in $\mt{1,1}$ with a large $j$-invariant then consists of $9$ points of multiplicity $1$ (where we introduced a contracted edge at the crossing), and one of multiplicity $3$ (where we introduced a contracted loop at the vertex of multiplicity $3$ --- due to realizability, this should again be the only possibility).

For a very small $j$-invariant, we do not have any contribution from the curves with a crossing. For the other, we can still attach the loop but let it be large, or we can introduce a small cycle by subdividing the triangle of area $3$ in the dual subdivision. By Kerber-Markwig, the $ev\times j$-multiplicity of the latter equals $9$. Again, if we shrink the loop to $0$, the two preimages degenerate to the same curve.

To sum up, the map $f$ has one preimage over the vertex which splits into two edges of weight $3$ and $9$, the edge of weight $3$ is an end, the edge of weight $9$ further splits until it becomes $9$ ends of weight $1$ over points with a very large $j$-invariant.

\section{Random observations yet to find a good place in the story.}
Anything in this section is at the level of musings or confusion, so I will not bother using the color blue.
\subsection{$\Mt{1,1}$ and a different tropicalization of $\overline{M}_{1,1}^{log}$?}\label{p24}

The moduli space $\overline{M}_{1,1}$ is isomorphic to the orbifold $\PP(4,6)$, with boundary structure given by one generic point (i.e. a point with isotropy group $\mu_2$). There are however two other interesting points, namely the two orbifold points with isotropy $\mu_4$ and $\mu_6$. Could one endow $\overline{M}_{1,1}$ with a logarithmic  structure consisting of these three points, and thus obtain a tropicalization which is a tripod which is not balanced in the standard way (but still balanced)? Could then one have some kind of forgetful morphism to $\Mt{1,1}$ and deduce a balancing condition for the vertex of $\Mt{1,1}$. Informally we would like to say that only morphisms from graphs to $\Mt{1,1}$ that approach the vertex with a weight which is a multiple of $12$ can be extended to harmonic morphisms over the ghost legs of the tripod. What would all I said mean in the log world?

\subsection{Torsion balancing and log-Pic?}
Our observations seem to suggest that the balancing on $\mt{1,1}$ should be described by assigning a sheaf of linear functions where the stalks over the open ray are $\ZZ$, whereas the stalk at the vertex is $\ZZ/12\ZZ$.
I would like to connect this to the classical fact that $Pic(\calM_{1,1}) = \ZZ/12\ZZ$ (a computation by Mumford that now can be recovered somewhat easily using orbifold technology). I believe that in Jonathan's magic point of view this is not a coincidence, there should be a connection between the sheaf of linear functions on a tropical object and the log-Pic of the log scheme of which the tropical object is a tropicalization of, but I am not knowledgeable enough to turn this into a real mathematical statement yet.

\subsection{Tropical Sections}\label{tsec}

Tropical sections are not really sections! In CCUW we show that the fact that a "tropical section" (as a morphism) is really a map $s_{i}:\mt{g,n}\times \RR \to \mt{g, n+1}$ should be taken seriously, as it is the natural corresponing object to a section in the logarithmic world.

Hence the codimension $1$ cones in the image of the section $s_i$ come as the images of:
\begin{itemize}
    \item $\sigma\times \{0\}$, where $\sigma$ is a top dimensional cone in $\mt{g,n}$. This corresponds to attaching the $n+1$-th leg at the vertex where the $i$-th legs is. These cones are horizontal, in the sense that they push forward to top dimensional cones of $\mt{g,n}$
    \item $\tau\times \RR $, where $\sigma$ is a top dimensional cone in $\mt{g,n}$. This amounts to replacing in tropical curves on each cone of codimension one the $i$-th leg with a  fork with ends $i$ and $n+1$.
    These cones are vertical, and hence they should push forward to $0$.
    \end{itemize}

In genus zero, we can already witness than the naive image  of $s_i$ (consisting only of the horizontal cones) is not a tropical cycle, as it is not balanced in $\mt{0,n+1}$.
One may however obtain a balanced tropical cycle by considering the cycle  a section to be a linear combination of both horizontal and vertical cones in the image of the section morphism. The horizontal cones come with multiplicity one, and the vertical cones come with a multiplcity which is the negative of the intersection number of $\psi_i$ with $\Delta_\tau$ (upstairs, this is the first Chern class of the one dimensional subbundle in the normal bundle to the stratum that consist in smooothing the new node).
    
    \begin{equation}\label{sec}
        [s_i] = [s_i(\sigma\times 0)] - \left(\int\Delta_\tau\cdot \psi_i\right) [s_i(\tau\times \RR)].
    \end{equation}
Let us check it for $s_1: \mt{0,4}\to \mt{0,5}$:
\begin{equation}
   [s_1] = D(125|34)+D(135|24)+D(145|23)- D(15|234).  
\end{equation}
This is indeed a balanced cycle in the natural embedding of $\mt{0,n}$ as a tropical compactification.

In fact, in genus $0$ this is always a balanced cycle:
First, notice that cones which are the image of $\sigma\times\{0\}$ --- we denote them by $\tilde{\sigma}$ --- have a $4$-valent vertex involving $i$ and $n+1$. Cones which are the image of $\tau\times\RR$ --- we denote them by $\tilde{\tau}$ --- have $i$, $n+1$ at a $3$-valent vertex and a $4$-valent vertex somewhere else.
The weight of such a $\tilde{\tau}$ as above is $0$ if the vertex adjacent to $i$, $n+1$ does not share a bounded edge with the $4$-valent vertex of $\tilde{\tau}$, and $-1$ otherwise. The weight of a cone $\tilde{sigma}$ is $1$.

A codimension one cone can either have 
\begin{itemize}
    \item another $4$-valent vertex somewhere, or
    \item a $5$-valent vertex involving $i$ and $n+1$, or
    \item a $5$-valent vertex adjacent to a bounded edge that is adjacent to $i$ and $n+1$.
\end{itemize}
In the first case, balancing holds as usual.
In the second case, let's call the sets of ends we can reach via the remaining three adjacent edges by $A$, $B$, $C$. We have four neighbours of the codimension one cone: The cone with a $4$-valent vertex with $A$, $B$, $C$, the cone with $A$ and $B$, the cone with $A$ and $C$, and the cone with $B$ and $C$. In the following sums, we let the index $S$ go over all $2$-element subsets of $[n]$ (i.e. we avoid $n+1$). By Kerber-Markwig-Psi, Lemma 2.7, the direction vector $v_{A\cup B\cup C}$ of the first cone satisfies:
\begin{align*}v_{A\cup B\cup C}= \sum_{S\subset A\cup B\cup C} v_S &= \sum_{S\subset A} v_S+ \sum_{S\subset B} v_S+\sum_{S\subset C} v_S\\&+\sum_{S, |S\cap (A\setminus B)|=1, |S\cap (B\setminus A)|=1} v_S \\&+\sum_{S, |S\cap (A\setminus C)|=1, |S\cap (C\setminus A)|=1} v_S\\&+\sum_{S, |S\cap (B\setminus C)|=1, |S\cap (C\setminus B)|=1} v_S.
\end{align*}
The first three summands are modded out, the remaining three are the generators of the other 3 cones, so with the weights as given above, balancing holds.

In the third case, let's call the sets of ends $A$, $B$, $C$, $D$ (with the fifth edge leading to $i$, $n+1$). We have six neighbours given by choices of two of the subsets that remain adjacent to the edge leading to $i$, $n+1$. These six cones are thus spanned by the vectors $v_{A\cup B}$, $v_{A\cup C}$, $v_{A\cup D}$, $v_{B\cup C}$, $v_{B\cup D}$, $v_{C\cup D}$. Their weights are all $-1$. Neglecting summands which are modded out anyway, we can, again using Lemma 2.7 of Kerber-Markwig-Psi, express $v_{A\cup B\cup C \cup D}$ (which is also $0$ when modding out) as the sum of $v_S$, where $S$ satisfies either $|S\cap (A\setminus B)|=1, |S\cap (B\setminus A)|=1$ or the analogue for each other choice of two of the sets. Sorting the summands with respect to th two sets, we obtain six summands that yield exactly the six generators above. So these six generators sum indeed up to $0$ and balancing holds.

Further, notice that with this definition of section, the relation
\begin{equation}\label{pb}
\psi_i = \pi_{n+1}^\ast\psi_i +[s_i]
\end{equation}
holds on the nose. 
In genus one, what if we define cycle sections to be balanced when defined as \eqref{sec}? What balancing does that impose on $\mt{1,n}$?
Here is a nice observation in $\mt{1,2}$. Consider the relation \eqref{pb}:
\begin{equation}
    \pi_{2}^\ast \psi_1 = \frac{1}{24}\tf 
\end{equation}
\begin{equation}
   [s_1] = \ts -\frac{1}{24}\tf 
\end{equation}
\begin{equation}
    \pi_{2}^\ast \psi_1 +[s_1] = \ts,
\end{equation}
which is the correct definition of tropical psi class if we believe that it should still coincide with the operational theory definition. So in conclusion, this definition of section cycle is what makes the pull back relation for psi classes recover the operational theory of psi classes in genus $1$.

\subsection{Operational theory vs. tropical cycles}
Put here also all computations and consistency checks for $\mt{1,2}$, as well as a comparison of the two  perspectives. Not sure we will ever need to use these formulas in the paper but I am tired to have to recompute everything every time I want to make a sanity check.

Operationally:
\begin{eqnarray}
\tv^{op} &=& 1/2\man +1\fish \\
  \ts^{op} &=& 0\ts +1/2 \tf \\
  \tf^{op} &=&  1\ts -(1/24) \tf\\
  \man^{op} &=& 1/2 \tv\\
  \fish^{op} &=& 1/2 1 \tv \\
  \ts^{op}\ts^{op}  &=& 0 \tv\\
  \ts^{op}\tf^{op}  &=& 1/2 \tv \\
  \tf^{op}\tf^{op} &=& -1/24 \tv
\end{eqnarray}

Introducing $\psi$ (as an operational class) into the mix:
\begin{eqnarray}
\psi &=& \ts \\
 \psi \ts^{op} &=& 1/2 \tv \\ 
 \psi \tf^{op} &=& 0 \tv \\
\end{eqnarray}

By inverting things we can make predictions about the values of the tropical intersections on the rays of $\mt{1,2}$:
\begin{eqnarray}
\ts &=& 1/12 \ts^{op}+\tf^{op}\\ 
\tf &=& 2\ts^{op}+0 \tf^{op}\\ 
\ts \ts &=& 1/24 \tv\\ 
\ts \tf &=& \tv \\ 
\tf \tf &=& 0 \tv \\ 
\end{eqnarray}
Note that the three last lines, which are computed going through the operational theory, are satisfying: the first recovers the degree of $\psi^2$ to be $1/24$, the second witnesses some sort of transversal intersection of the rays, and the third shows that the tropical fiber can be moved off itself.

As a final remark in this section, the operational theory of tropical $\psi$ classes has the $\mt{1,1}$ as a special case, but other than that it parallels the genus zero theory in the sense that $\psi_i$ may be described as the sum of all codimension one cones representing tropical curves where all vertices are rational and the $i$-th mark lies on the unique four-valent vertex.
\subsection{All classical facts that we want to recover or parallel}

Here is a list of top 

\begin{enumerate}
\item Pull-back relation 
\item String
\item Dilaton
\item Intersection with strata
\item Non-transversal intersections of strata
\item Formulas for top intersections
\end{enumerate}

\section{Example computation of the self-intersection of a section}

\subsection{$c_1$ of a tropical line bundle on tropical $\PP^1$}

Consider the closed interval $X = [-\infty, \infty]$ as a model of tropical $\PP^1$.
We have a sheaf $Aff_X$ (playing the role of $\mathcal{O}_X^\ast$) of affine linear functions defined by:
\begin{eqnarray}
 Aff_X (\  (a,b) \ )   \cong \bZ \times \R & = \{ mx +r| m\in \bZ, r\in \R\}, \nonumber \\
  Aff_X (\  [-\infty ,b) \ )     \cong \R & = \{ r| r\in \R\}, \nonumber \\
    Aff_X (\  (a, \infty] \ )   \cong  \R & = \{ r|  r\in \R\}, \nonumber \\
      Aff_X (\  [-\infty ,\infty] \ ) \times \R & = \{ r|  r\in \R\}.
 \end{eqnarray}
 
 Note that we consider the functions $mx +r$ to have a zero of order $m$ at $-\infty$, and similarly the functions $-mx +r$ to have a zero of order $m$ at $\infty$.
 The only global affine functions on $\PP^1$ are the constants.
 
 A {\bf line bundle}  is obtained by gluing together local trivialization via affine functions. As usual, we can cover $\PP^1$ with two charts:
 \begin{description}
 \item[$U_{-\infty} = $] $ [-\infty, \infty)$,
  \item[$U_{\infty} = $]$ (-\infty, \infty]$, so that the intersection is
   \item[$U_{-\infty}\cap U_{\infty}  = $]$ (-\infty, \infty)$.
 \end{description}
As in classical algebraic geometry, an isomorphism class of a line bundle is identified by a cocycle $kx$, corresponding to gluing the two local trivializations via  $y_{\infty } = kx +y_{-\infty}$, for $k\in \bZ$. We are free to ignore the real translation factor since translations are global affine functions, and so two cocycles differing by a translation give isomorphic line bundles. We denote $\mathcal{O}(-k)$ the line bundle given by the cocycle $kx$.

The regular sections of the line bundle $\mathcal{O}(d)$ (for $d\geq 0$)  having zeros only at $\pm \infty$ are:
$$
 \{ (y_{-\infty}= mx+r,y_{\infty}= (m-d)x+r) | 0\leq m\leq d, r\in \R \}.
$$

An example of a global section having a zero of order $d$ at the point $0$ is given by:
$$
 \left( y_{-\infty}= \left\{\begin{array}{cl}0 & x\in [-\infty,0]\\ dx & x\in [0,\infty]\\ \end{array}\right.,y_{\infty}=  \left\{\begin{array}{cl}-dx & x\in [-\infty,0]\\ 0 & x\in [0,\infty]\\ \end{array}\right.\right ).
$$

In general, a regular section of $\mathcal{O}(d)$ can be identified  with  a monotonic increasing  piecewise linear function on the chart $U_{-\infty}$ which starts at $-\infty$ with some non-negative integral slope, and arrives at $\infty$ with slope less than or equal to $d$. The zeros of such a section are given by the points where a change of slope happens, together with $\pm \infty$ if the slope there is not $0$ (at $-\infty$) or $d$ (at $\infty$). The multiplicities are computed as change of slopes going from left to right, where a function on the chart 
$U_{-\infty}$ is regular at $-\infty$ if it has slope $0$ and it is regular at $\infty$ if it has slope $d$.
One can see that the sum of the multiplicities of the zeroes of a regular section of $\mathcal{O}(d)$ is $d$, and therefore we define $c_1(\mathcal{O}(d)) = d[pt.]$
It is now straightforward to introduce meromorphic sections, multiplicities of poles, and define $c_1$ also for negative line bundles.
\subsection{A family of elliptic curves}
We describe a family $X$ of elliptic curves over $\PP^1 = [-\infty, \infty]$. As a cone complex, this is the union of four plane (extended) orthants, let us called them $L_{\pm}, S_{\pm}$.
The one dimensional faces of  $L_-$ are identified, and glued with the horizontal axis of $S_{-}$ (and similarly for the $+$). The vertical axes of  $S_-$ and $S_+$ are identified.
Vertical projection in the $S_{\pm}$ orthants and diagonal projection in the $L_{\pm}$ orthants give a map  $\pi: X \to \PP^1 = [-\infty, \infty]$ whose fibers are elliptic curves.
To make this cone complex into a tropical object, we must endow it with a sheaf of affine linear functions. We define:
\begin{eqnarray}
 Aff_X (\ \pi^{-1} (a,b) \ )   \cong \bZ \times \R & = \{ mx +r| m\in \bZ, r\in \R\}, \nonumber \\
  Aff_X (\ \pi^{-1} [-\infty ,b) \ )   \cong \R & = \{ r|  r\in \R\}, \nonumber \\
    Aff_X (\  \pi^{-1}(a, \infty] \ )   \cong  \R & = \{r| r\in \R\}, \nonumber \\
      Aff_X (\  \pi^{-1}[-\infty ,\infty] \ ) \cong \R & = \{ r|  r\in \R\}.
 \end{eqnarray}
 I.e. for all inverse images of open sets from the base the affine functions are the same (this is saying $\pi_\ast (Aff_X) = Aff_{\PP^1}$).
 
 If $U = (S_-\cup L_-) \smallsetminus \Delta_L$ , where $\Delta_L$ consists of the diagonal of $L_-$, then 
 $$
 Aff_X(U) \cong   (\bZ \oplus \bZ \oplus \bZ) \times \R  = \{ mx+ (ay_1+by_2 +c y_3)+r| m, a, b, c\in \bZ, a+b+c = 0,  r\in \R\},
 $$
where $y_1$ is the vertical coordinate on $S_-$, $y_2$ and $y_3$ are the two coordinates on $L_-$ appropriately restricted to each of the two halves so that are normal to the seam of the flap. This is essentially saying that $U$ is identified with the product of $[-\infty, 0]$ with a standard tripod in the plane.
Finally consider $U = (S_-\cup S_+)\smallsetminus \{boundary\}$. Denote by $(x_-, y_-)$ the coordinates on $S_-$ and similarly for $+$.
\begin{align}
 Aff_X(U) \cong   (\bZ \oplus \bZ ) \times \R  &= \{ m_-x_-+ n_-y_-+r | m_-,n_- \in \bZ,  r\in \R\} \nonumber \\
  &= \{ m_+x_++ n_+y_++r | m_+,n_+ \in \bZ,  r\in \R\}.
\end{align}
In other words, affine functions on $U$ can be determined by what they are on either flap, but part of the datum that MUST be given is  how to transition  from one chart to the other: so we add the information that
\begin{equation}\label{tf}
x_+ = -x_- \ \ \ \ \ \ \  y_+= y_- - Ax_-,
\end{equation}

If now we want to include the infinity section in our open set $U$, we have
\begin{align}
 Aff_X(U) \cong   (\bZ ) \times \R  &= \{ m_-x_-+r | m_-\in \bZ,  r\in \R\} \nonumber \\
  &= \{ m_+x_++r | m_+\in \bZ r\in \R\}.
\end{align}
Including some of the vertical infinity faces  will amount to restrict to zero the $m$  slopes.

for $A$ in $\bZ$. If now we use the coordinates $(x_+, y_+)$ to embed $U$ into (an extended) $\R^2$, we have that the + flap maps identically to the first orthant, but the $-$ flap is mapped to the plane by the linear function $(1,0) \mapsto (-1, -A), (0,1) \mapsto (0,1)$.  Figure \ref{fam} depicts this local embedding for  the two cones $S_\pm$, while the cones $L_\pm$ which are self-glued do not communicate with such an embedding. We depicted them in the picture just to have  an idea of the global topology of the family.  
What we described essentially describes the affine functions on $X$ completely. It is easy to further localize to smaller open sets and figure out what the answer should be.

\begin{figure}[h]
\begin{center}
\begin{tikzpicture}
\begin{scope}[scale = 0.5]
\draw[very thick, fill = yellow] (0,0) -- (0,8.5)--(8.5,8.5) -- (8.5,0) --(0,0);
\draw[very thick, fill = yellow] (0,0) -- (0,8.5)--(-8.5,8.5) -- (-8.5,-8.5) --(0,0);
\draw[very thick, red] (-8.5,8.5) -- (8.5,8.5) ;
\draw[->] (-8,0)-- (8,0);
\draw[->] (0,-8)-- (0,8);
\draw[very thick, fill = orange] (0,0)-- (8.5,0)--(8.5,-4.05) --(0,0);
\draw[very thick, fill = gray] (8.5,-2) ellipse (1 and 2);

\draw[very thick, fill = orange] (0,0)-- (-8.5,-8.5)--(-8.2,-12.5) --(0,0);
\draw[very thick, fill = gray] (-8.5,-10.5) ellipse (1 and 2);
 \foreach \i in {-8,...,8}
      \foreach \j in {0,...,8}{
        \draw[fill = red] (\i,\j) circle(1pt);};

 \foreach \i in {-8,...,0}
      \foreach \j in {\i,...,0}{
        \draw[fill = red] (\i,\j) circle(1pt);};

\node at(4,4) {$S_+$};
\node at(-4,4) {$S_-$};
\node at(4,-1) {$L_+$};
\node at(-4,-5) {$L_-$};
\node[red] at(9,8.5) {$s_\infty$};

 \end{scope}
\end{tikzpicture}
\caption{The family $X$. The yellow part shows the local embedding dictated by the sheaf of affine functions. In this case $A = 1$. In red we see the image of the section $s_\infty$.}
\label{fam}
\end{center}
\end{figure}

\subsection{The self-intersection of $s_\infty$}

We now consider the section $s_\infty$ defined by $s_\infty (x) = (x, \infty)$ for every  $x\in [-\infty, +\infty]$. First off, we want to show that the image of $s_\infty$, with weight one, is a Cartier divisor on $X$.
Cover $X$ with three open sets, $|X = X \smallsetminus \{(-\infty, \ast)\} , X| = X \smallsetminus \{(+\infty, \ast)\}$ and $\overline{X} = X \smallsetminus \{(\ast, \infty)\}$: each of these three sets is  obtained by removing the line at infinity in the position indicated  by the bar in the notation.
Then the Cartier divisor $[D_{s_\infty}]$ is given by the data:
$$
[D_{s_\infty}] = \left( (\overline{X}, 0), ({{\color{red}|}X}, -y_-), ({X{\color{red}|}}, -y_+)\right).
$$

The difference of the meromorphic functions $0, y_-, y_+$ in the double overlaps are affine functions. This is obvious for $y_- = 0-y_-, y_+$. The result is given for $-y_++y_-$ by  formula   \eqref{tf}. Note that the set ${{\color{red}|}X}\cap {X{\color{red}|}}$ contains the infinity section and the zero section, so having slope $0$  in the $y$ direction is essential for the transition being affine in the intersection.

We are pretty close to being done at this point. We want to define $s_\infty^2:= s_\infty^\ast(D_{s_\infty})$, but if we just naively pull back the meromorphic functions giving the Cartier data, we end up getting the constant function equal to $\infty$ everywhere. That is not very good.
So we make one extra, natural step. We consider the line bundle given by the Cartier data: this is identified by the Chech cocycle corresponding to the difference or the restriction of the meromorphic functions giving the Cartier data, i.e.:
$$
L_{D_{s_\infty}} =  \left( (\overline{X} \cap {{\color{red}|}X} , y_-), (\overline{X} \cap {X{\color{red}|}}, -y_+), ({{\color{red}|}X}\cap {X{\color{red}|}}, -Ax_+)\right).
$$ 
The pull-back of this line bundle can now be done:
\begin{align}
s_\infty^\ast L_{D_{s_\infty}} &=  \left( (s_\infty^\ast(\overline{X} \cap {{\color{red}|}X}) , s_\infty^\ast(y_-), ( s_\infty^\ast(\overline{X} \cap {X{\color{red}|}}),  s_\infty^\ast(-y_+)), ( s_\infty^\ast({{\color{red}|}X}\cap {X{\color{red}|}}),  s_\infty^\ast(-Ax_+))\right)\nonumber \\
& = ([-\infty,\infty)\cap (-\infty, \infty], -Ax)
\end{align}
There is only one double intersection since the other two don't intersect the image of the section $s_\infty$.
But we have obtained the cocycle for the line bundle $\mathcal{O}_{\PP^1}(A)$. Therefore:
$$
s_\infty^2:= c_1(s_\infty^\ast (L_{D_{s_\infty}}) ) =  c_1(\mathcal{O}_{\PP^1}(A))  = A[pt.]
$$
\section{$16$ vs. $18$}

I want to discuss the computation of $\psi_1$ on a one dimensional family of genus $1$ curves in $\PP^1\times \PP^1$ of bidegree $(3,2)$. We have been guess-puting the tropical computation and found that it seems hard to obtain the answer we want ($16$), where it seems somewhat natural to obtain $18$ as an answer. I believe that what this means is that we are in fact not computing the $\psi$ class pulled back from the moduli space of curves, but instead the $\psi$ class on the moduli space of stable maps.

Here are some preliminary facts:

$$[C]:= \prod_{i=1}^9 ev^{\ast}_i([pt.])\subset \overline{M}_{1,9}(\PP^1\times \PP^1, (3,2))$$
is a curve class in the moduli space of stable maps that may be represented by the curve of maps of genus $1$ whose marked points are mapped to $9$ fixed points in general position.
We have the following natural diagram:
$$
\xymatrix{
C \ar[r]^{\hspace{-1cm} \iota} \ar[dr]_{96}\ \ \ \ \ & 
\ar[d]_\mu \overline{M}_{1,9}(\PP^1\times \PP^1, (3,2))\\
    & \overline{M}_{1,1}.}
$$

We have the fundamental relation:
$$
\psi_1 = \mu^\ast(\psi_1)+ D_1,
$$
where $D_1$ consists of the divisor of stable maps where the mark $1$ is on a genus zero component which attaches at one point to the genus one component.

We can now compute:
$$
C\cdot \psi_1 = C\cdot(\mu^\ast(\psi_1)+D_1).
$$

From Dhruv-Yoav, or Ravi (https://arxiv.org/pdf/alg-geom/9709003.pdf, page 11) we know that the degree of the map $\mu\circ \iota$ equals $96$, from which we obtain
$$
16 = C\cdot(\mu^\ast(\psi_1)).
$$

We now compute $C\cdot D_1 = 2$ as follows: there is a curve $X$ of class $(3,2)$ that represents the image of a map in $C\cdot D_1$: it consists of the horizontal (class $(1,0)$) line $L$ through the point $P_1$ union the unique genus one curve $E$ of class $(2,2)$ through the remaining $8$ points. We note that $L$ and $E$ intersect in two points because of Bezout's theorem. Which means that there are two maps whose image is $X$: you may attach the rational component of the source to either points of intersection of $E$ with $L$.

We finally have established
$$
C\cdot \psi_1 = C\cdot(\mu^\ast(\psi_1)+D_1) = 16+2 = 18.
$$
